# Supplementary material for: Transposer: Universal Texture Synthesis Using Feature Maps as Transposed Convolution Filter
Source: arXiv:2007.07243 source file (2020-07-14)
Supplement: Supplementary file 1 [file suppl_content.tex]

\section*{Appendix}

\subsection*{Framework Detail}

% \subsubsection*{Animation of Computing Self-Similarity Map \& Transpose Convolution Operation}

% Please check the animation video of how to compute self-similarity map and do the transpose convolution operation.
% % We provide an animation video of how we compute self-similarity map and how the transpose convolution operation is done. Please check the animation video for more details.

\subsubsection*{Transpose Convolution Block}

Figure~\ref{fig:transconv_block} shows the details for transpose convolution block in our framework. Table~\ref{tab:transconvdiff} lists the main differences between typical transpose convolution operation and our transpose convolution operation.
\begin{figure}[h]
    \centering
    \includegraphics[width=0.75\textwidth]{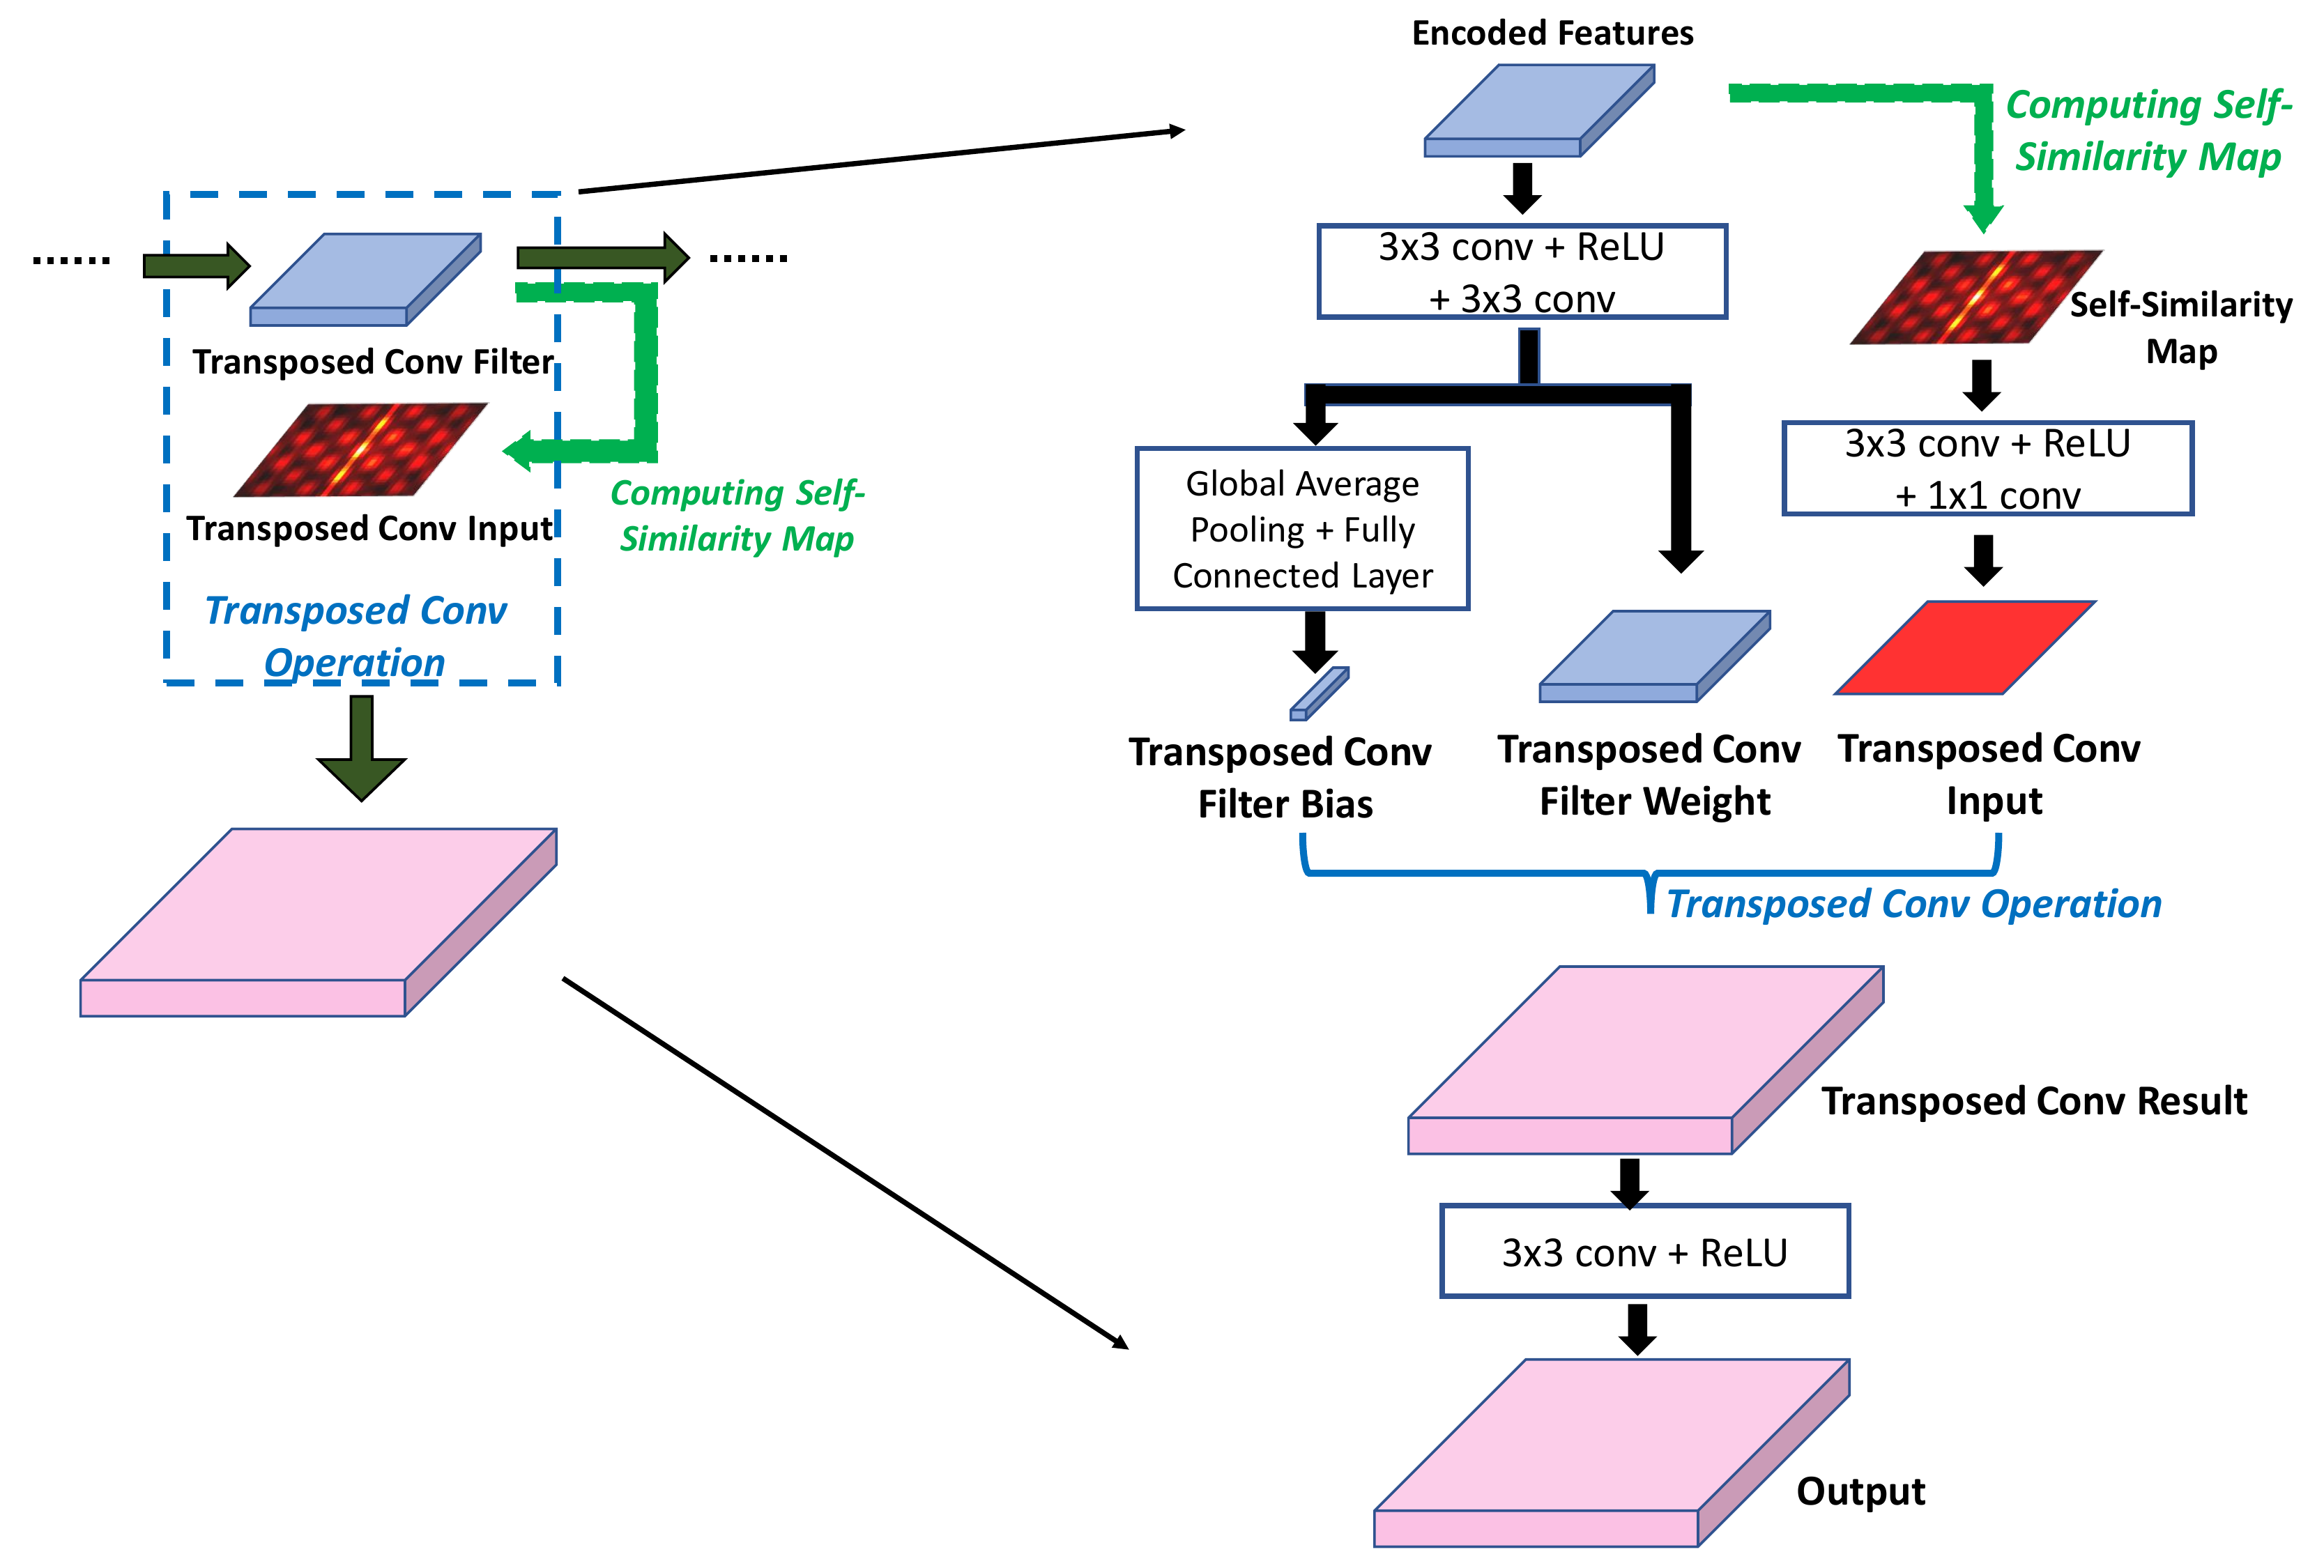}
    \caption{The details of a transpose convolution block. The left part shows the corresponding preview which is used in the Figure 3 in the main paper; the right part shows the details of this transpose convolution block.}
    \label{fig:transconv_block}
\end{figure}

\begin{table}[h]
    \centering
    \begin{tabular}{l|l|l}
    \multicolumn{1}{c}{} & typical transpose conv operation & our transpose conv operation \\
    \hline
    input & output from previous layer & self-similarity map from encoded features \\
    filter & learn-able parameters & feature maps from encoder \\
    bias term & learn-able parameters & averaged pooling of encoded features followed by linear transform \\
    filter size & small (e.g. 4x4, 3x3) & large (e.g. 8x8, 16x16, 32x32, 64x64) \\
    stride & 2(for upsampling purpose) & 1 \\
    \end{tabular}
    \addtolength{\tabcolsep}{3pt}
    \vspace{2mm}
    \caption{Main differences between typical transpose convolution and our transpose convolution operation}
    \label{tab:transconvdiff}
    \vspace{-2mm}
\end{table}

\subsubsection*{Network Details}
Table~\ref{tab:net_detail} shows the details of generator. The discriminator network is the same with pix2pixHD's.

\begin{table}
    \centering
    \scalebox{0.6}{
    \begin{tabular}{c|c|c|c|c|c|c}
         & Block & Filter Size & \# Filters & Stride/UpSample Factor & SyncBatchNorm & ReLU\\
        \hline
        \hline
         \multirow{9}{*}{Encoder} & Conv1& 3$\times$3& 3 $\rightarrow$ 64& 1& Y& Y\\
         & Conv2\_1& 3$\times$3& 64 $\rightarrow$ 128& 2& Y& Y\\
         & Conv2\_2& 3$\times$3& 128 $\rightarrow$ 128& 1& Y& Y\\
         & Conv3\_1& 3$\times$3& 128 $\rightarrow$ 256& 2& Y& Y\\
         & Conv3\_2& 3$\times$3& 256 $\rightarrow$ 256& 1& Y& Y\\
         & Conv4\_1& 3$\times$3& 256 $\rightarrow$ 512& 2& Y& Y\\
         & Conv4\_2& 3$\times$3& 512 $\rightarrow$ 512& 1& Y& Y\\
         & Conv5\_1& 3$\times$3& 512 $\rightarrow$ 1024& 2& Y& Y\\
         & Conv5\_2& 3$\times$3& 1024 $\rightarrow$ 1024& 1& Y& Y\\
         \hline
         \hline
        \multirow{7}{*}{TransConv\_Block3 (w/ Conv3\_2)}  & FilterBranch\_Conv1 & 3$\times$3 & 256 $\rightarrow$ 256 & 1 & - & Y \\
        & FilterBranch\_Conv2 & 3$\times$3 & 256 $\rightarrow$ 256 & 1 & - & - \\
        & FilterBranch\_FC1 & - & 256 $\rightarrow$ 256 & 1 & - & - \\
        & SelfSimilarityMapBranch\_Conv1 & 3$\times$3 & 1 $\rightarrow$ 8 & 1 & - & Y \\
        & SelfSimilarityMapBranch\_Conv2 & 3$\times$3 & 8 $\rightarrow$ 1 & 1 & - & - \\
        & Transpose Convolution Operation & $\frac{\text{orig\_H}}{4}\times \frac{\text{orig\_W}}{4}$ & filter: 256, input: 1 $\rightarrow$ 256 & - & - & - \\
        & OutputBranch\_Conv & 3$\times$3 & 256 $\rightarrow$ 256 & 1 & - & Y \\
        \hline
        \multirow{7}{*}{TransConv\_Block4 (w/ Conv4\_2)}  & FilterBranch\_Conv1 & 3$\times$3 & 512 $\rightarrow$ 512 & 1 & - & Y \\
        & FilterBranch\_Conv2 & 3$\times$3 & 512 $\rightarrow$ 512 & 1 & - & - \\
        & FilterBranch\_FC1 & - & 512 $\rightarrow$ 512 & 1 & - & - \\
        & SelfSimilarityMapBranch\_Conv1 & 3$\times$3 & 1 $\rightarrow$ 8 & 1 & - & Y \\
        & SelfSimilarityMapBranch\_Conv2 & 3$\times$3 & 8 $\rightarrow$ 1 & 1 & - & - \\
        & Transpose Convolution Operation & $\frac{\text{orig\_H}}{8}\times \frac{\text{orig\_W}}{8}$ & filter: 512, input: 1 $\rightarrow$ 512 & - & - & - \\
        & OutputBranch\_Conv & 3$\times$3 & 512 $\rightarrow$ 512 & 1 & - & Y \\
        \hline
        \multirow{5}{*}{TransConv\_Block5 (w/ Conv5\_2)}  & FilterBranch\_Conv1 & 3$\times$3 & 1024 $\rightarrow$ 1024 & 1 & - & Y \\
        & FilterBranch\_Conv2 & 3$\times$3 & 1024 $\rightarrow$ 1024 & 1 & - & - \\
        & FilterBranch\_FC1 & - & 1024 $\rightarrow$ 1024 & 1 & - & - \\
        & SelfSimilarityMapBranch\_Conv1 & 3$\times$3 & 1 $\rightarrow$ 8 & 1 & - & Y \\
        & SelfSimilarityMapBranch\_Conv2 & 3$\times$3 & 8 $\rightarrow$ 1 & 1 & - & - \\
        & Transpose Convolution Operation & $\frac{\text{orig\_H}}{16}\times \frac{\text{orig\_W}}{16}$ & filter: 1024, input: 1 $\rightarrow$ 1024 & - & - & - \\
        & OutputBranch\_Conv & 3$\times$3 & 1024 $\rightarrow$ 1024 & 1 & - & Y \\
        \hline
        \hline
         \multirow{11}{*}{Decoder} & BilinearUpSample1(w/ TransConv\_Block5 output)& - & - & 2 & - & -\\
         & Conv6& 3$\times$3& 1024 $\rightarrow$ 512& 1& Y& Y\\
         & Sum (Conv6 + TransConv\_Block4 output) & - & - &  - & - & -\\
         & BilinearUpSample2 & - & - & 2 & - & -\\
         & Conv7& 3$\times$3& 512 $\rightarrow$ 256& 1& Y& Y\\
         & Sum (Conv7 + TransConv\_Block3 output) & - & - &  - & - & -\\
         & BilinearUpSample3 & - & - & 2 & - & -\\
         & Conv8& 3$\times$3& 256 $\rightarrow$ 128& 1& Y& Y\\
         & BilinearUpSample4 & - & - & 2 & - & -\\
         & Conv9& 3$\times$3& 128 $\rightarrow$ 64& 1& Y& Y\\
         & Conv10& 3$\times$3& 64 $\rightarrow$ 3& 1 & - & -\\
         \hline
    \end{tabular}
    }
    \vspace{2mm}
    \caption{The details of network parameters. TransConv\_Block3-5 represent the three transpose convolution blocks in our framework (The diagrams can be found in Figure 3 in the main paper and Figure~\ref{fig:transconv_block}). SyncBatchNorm column indicates Synchronized Batch Normalization layer after Conv. ReLU column shows whether ReLU is used (following the SyncBatchNorm if SyncBatchNorm is used). BilinearUpSample represents bilinear upsampling. Sum denotes the simple summation. \text{orig\_H} and \text{orig\_W} are input image's height and width.}
    \label{tab:net_detail}
\end{table}

\clearpage
\subsection*{Additional Comparison}

\subsubsection*{128 to 256 Synthesis}

\noindent\textbf{Non-stat. and Non-stat.$^{*}$ baselines}: we take the original code from the author's github repository. The original training strategy for each training iteration is: 1). randomly crop a $2H \times 2W$ from the original big image($>2H \times 2W$) as the target image; 2). from the target image, randomly crop a $H \times W$ image as the input image. Thus, for 128 to 256 synthesis, to train Non-stat. (without seeing ground truth $256 \times 256$ image), for each training iteration, we randomly crop a $96 \times 96$ image from the input $128 \times 128$ image as target image then from the target image, we randomly crop a $48 \times 48$ image as input.  To train Non-stat.* (with directly seeing ground truth $256 \times 256$ image), for each training  iteration, we randomly crop a $128 \times 128$ image from the ground truth $256 \times 256$ image as the target image and then from the target image, we randomly crop a $64 \times 64$ image as input image. For both Non-stat. and Non-stat.*, the inference stage will take $128 \times 128$ image as input.

\noindent\textbf{sinGAN and sinGAN$^{*}$ baselines}: for training with sinGAN, we used the original author's implementation available on github. And we used the default settings the author provided in their source code. sinGAN code can synthesize textures in two different modes, one that generates a random variation which is of the same size as input texture (we directly using ground truth $256\times256$ for training, denoted as sinGAN$^{*}$), and another that generates a texture of larger size (only using $128\times128$ image, denoted as sinGAN).

% comparison images
\begin{figure}[h]
\centering
\scalebox{0.6}{
% \addtolength{\tabcolsep}{-4pt}   
\begin{tabular}{c|cccccccc}
\multicolumn{1}{c}{} & \multicolumn{8}{c}{} \\
input & ours & Self-tuning & pix2pixHD & WCT & sinGAN$^{(*)}$ & Non-stat.$^{(*)}$ & DeepTexture & ground truth \\
\hline
\hline
\includegraphics[width=0.07\textwidth]{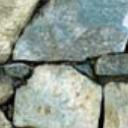} &
\includegraphics[width=0.14\textwidth]{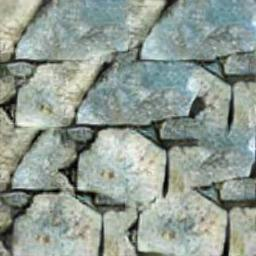} &
\includegraphics[width=0.14\textwidth]{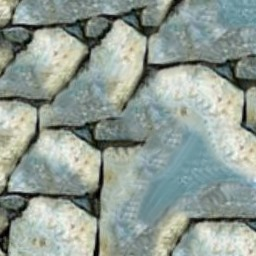} &
\includegraphics[width=0.14\textwidth]{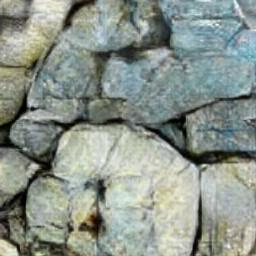} &
\includegraphics[width=0.14\textwidth]{Compare/WCT/DSC_0828_target_iter3_alpha_100.jpg} &
\includegraphics[width=0.14\textwidth]{Compare/singan/DSC_0828_input.jpg} &
\includegraphics[width=0.14\textwidth]{Compare/nonstationary/DSC_0828.jpg} &
\includegraphics[width=0.14\textwidth]{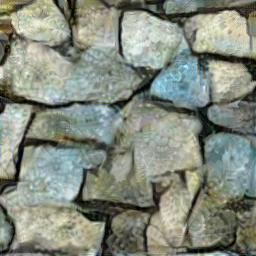} &
\includegraphics[width=0.14\textwidth]{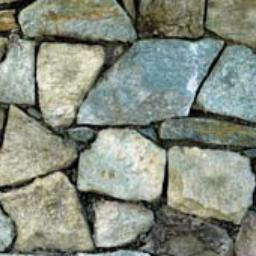} \\
\hline
\hline

\includegraphics[width=0.07\textwidth]{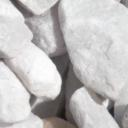} &
\includegraphics[width=0.14\textwidth]{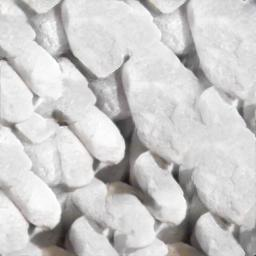} &
\includegraphics[width=0.14\textwidth]{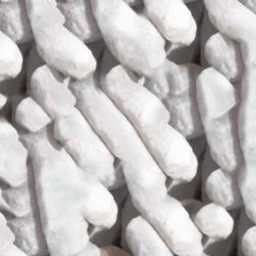} &
\includegraphics[width=0.14\textwidth]{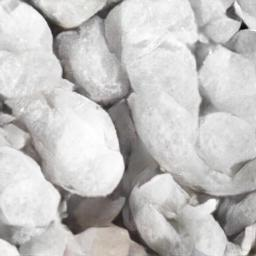} &
\includegraphics[width=0.14\textwidth]{Compare/WCT/117_c1l4r120_target_iter3_alpha_100.jpg} &
\includegraphics[width=0.14\textwidth]{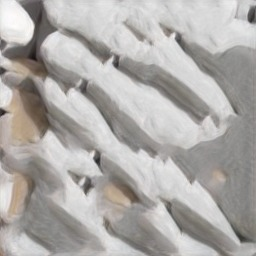} &
\includegraphics[width=0.14\textwidth]{SupplCompare/nonstationary_noGT/117_c1l4r120.jpg} &
\includegraphics[width=0.14\textwidth]{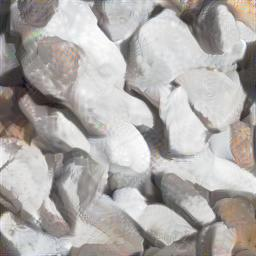} &
\includegraphics[width=0.14\textwidth]{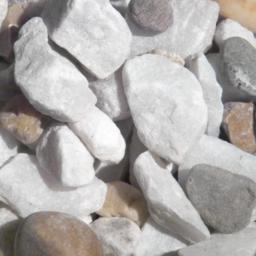} \\
\includegraphics[width=0.07\textwidth]{SupplCompare/TransConv/52_c3l3r180_input.jpg} &
\includegraphics[width=0.14\textwidth]{SupplCompare/TransConv/52_c3l3r180_output.jpg} &
\includegraphics[width=0.14\textwidth]{SupplCompare/SelfTune/52_c3l3r180_input.jpg} &
\includegraphics[width=0.14\textwidth]{SupplCompare/pix2pixHD/52_c3l3r180_output.jpg} &
\includegraphics[width=0.14\textwidth]{SupplCompare/WCT/52_c3l3r180_target_iter3_alpha_100.jpg} &
\includegraphics[width=0.14\textwidth]{SupplCompare/singan/52_c3l3r180.jpg} &
\includegraphics[width=0.14\textwidth]{SupplCompare/nonstationary_noGT/52_c3l3r180.jpg} &
\includegraphics[width=0.14\textwidth]{SupplCompare/deeptexture/52_c3l3r180.jpg} &
\includegraphics[width=0.14\textwidth]{SupplCompare/TransConv/52_c3l3r180_target.jpg} \\
\includegraphics[width=0.07\textwidth]{SupplCompare/TransConv/5_c3l5r120_input.jpg} &
\includegraphics[width=0.14\textwidth]{SupplCompare/TransConv/5_c3l5r120_output.jpg} &
\includegraphics[width=0.14\textwidth]{SupplCompare/SelfTune/5_c3l5r120_input.jpg} &
\includegraphics[width=0.14\textwidth]{SupplCompare/pix2pixHD/5_c3l5r120_output.jpg} &
\includegraphics[width=0.14\textwidth]{SupplCompare/WCT/5_c3l5r120_target_iter3_alpha_100.jpg} &
\includegraphics[width=0.14\textwidth]{SupplCompare/singan/5_c3l5r120.jpg} &
\includegraphics[width=0.14\textwidth]{SupplCompare/nonstationary_noGT/5_c3l5r120.jpg} &
\includegraphics[width=0.14\textwidth]{SupplCompare/deeptexture/5_c3l5r120.jpg} &
\includegraphics[width=0.14\textwidth]{SupplCompare/TransConv/5_c3l5r120_target.jpg} \\
\includegraphics[width=0.07\textwidth]{SupplCompare/TransConv/31_c3l2r60_input.jpg} &
\includegraphics[width=0.14\textwidth]{SupplCompare/TransConv/31_c3l2r60_output.jpg} &
\includegraphics[width=0.14\textwidth]{SupplCompare/SelfTune/31_c3l2r60_input.jpg} &
\includegraphics[width=0.14\textwidth]{SupplCompare/pix2pixHD/31_c3l2r60_output.jpg} &
\includegraphics[width=0.14\textwidth]{SupplCompare/WCT/31_c3l2r60_target_iter3_alpha_100.jpg} &
\includegraphics[width=0.14\textwidth]{SupplCompare/singan/31_c3l2r60.jpg} &
\includegraphics[width=0.14\textwidth]{SupplCompare/nonstationary/31_c3l2r60.jpg} &
\includegraphics[width=0.14\textwidth]{SupplCompare/deeptexture/31_c3l2r60.jpg} &
\includegraphics[width=0.14\textwidth]{SupplCompare/TransConv/31_c3l2r60_target.jpg} \\
\includegraphics[width=0.07\textwidth]{SupplCompare/TransConv/112_c3l4r180_input.jpg} &
\includegraphics[width=0.14\textwidth]{SupplCompare/TransConv/112_c3l4r180_output.jpg} &
\includegraphics[width=0.14\textwidth]{SupplCompare/SelfTune/112_c3l4r180_input.jpg} &
\includegraphics[width=0.14\textwidth]{SupplCompare/pix2pixHD/112_c3l4r180_output.jpg} &
\includegraphics[width=0.14\textwidth]{SupplCompare/WCT/112_c3l4r180_target_iter3_alpha_100.jpg} &
\includegraphics[width=0.14\textwidth]{SupplCompare/singan/112_c3l4r180.jpg} &
\includegraphics[width=0.14\textwidth]{SupplCompare/nonstationary/112_c3l4r180.jpg} &
\includegraphics[width=0.14\textwidth]{SupplCompare/deeptexture/112_c3l4r180.jpg} &
\includegraphics[width=0.14\textwidth]{SupplCompare/TransConv/112_c3l4r180_target.jpg} \\
\includegraphics[width=0.07\textwidth]{SupplCompare/TransConv/BrickSmallBrown0118_350_input.jpg} &
\includegraphics[width=0.14\textwidth]{SupplCompare/TransConv/BrickSmallBrown0118_350_output.jpg} &
\includegraphics[width=0.14\textwidth]{SupplCompare/SelfTune/BrickSmallBrown0118_350_input.jpg} &
\includegraphics[width=0.14\textwidth]{SupplCompare/pix2pixHD/BrickSmallBrown0118_350_output.jpg} &
\includegraphics[width=0.14\textwidth]{SupplCompare/WCT/BrickSmallBrown0118_350_target_iter3_alpha_100.jpg} &
\includegraphics[width=0.14\textwidth]{SupplCompare/singan/BrickSmallBrown0118_350.jpg} &
\includegraphics[width=0.14\textwidth]{SupplCompare/nonstationary_noGT/BrickSmallBrown0118_350.jpg} &
\includegraphics[width=0.14\textwidth]{SupplCompare/deeptexture/BrickSmallBrown0118_350.jpg} &
\includegraphics[width=0.14\textwidth]{SupplCompare/TransConv/10_c1l5r120_target.jpg} \\
\includegraphics[width=0.07\textwidth]{SupplCompare/TransConv/10_c1l5r120_input.jpg} &
\includegraphics[width=0.14\textwidth]{SupplCompare/TransConv/10_c1l5r120_output.jpg} &
\includegraphics[width=0.14\textwidth]{SupplCompare/SelfTune/10_c1l5r120_input.jpg} &
\includegraphics[width=0.14\textwidth]{SupplCompare/pix2pixHD/10_c1l5r120_output.jpg} &
\includegraphics[width=0.14\textwidth]{SupplCompare/WCT/10_c1l5r120_target_iter3_alpha_100.jpg} &
\includegraphics[width=0.14\textwidth]{SupplCompare/singan/10_c1l5r120.jpg} &
\includegraphics[width=0.14\textwidth]{SupplCompare/nonstationary_noGT/10_c1l5r120.jpg} &
\includegraphics[width=0.14\textwidth]{SupplCompare/deeptexture/10_c1l5r120.jpg} &
\includegraphics[width=0.14\textwidth]{SupplCompare/TransConv/10_c1l5r120_target.jpg} \\
\end{tabular}
}
\caption{Results of different approaches on 128 to 256 texture synthesis. For sinGAN($^{*}$) Non-stat.$^{(*)}$ results, the first row show the results of training with ground truth; the rest rows show the results of training without ground truth. (Training with ground truth means using the ground truth 256$\times$256 image as the target for each training iteration.) WCT and DeepTexture directly take ground truth images as inputs.}
\label{fig:result256}
\end{figure}

\clearpage

\subsubsection*{256 to 512 Synthesis}

In Table~\ref{tab:eval256to512}, we provide the quantitative comparisons for the synthesis results of 256 to 512. Figure~\ref{fig:result512} shows more visual comparisons of different approaches. 

\begin{table}[h]
\centering
\scalebox{1.2}{
    \begin{tabular}{l|ccccc}
    \multicolumn{1}{c}{} & \multicolumn{1}{|c}{SSIM} & FID & c-FID & LPIPS & c-LPIPS \\
    \hline
    \hline
    % Naive tiling &  &  &  &  &  \\
    Self-tuning & 0.3157 & 95.829 & 0.4393 & 0.4078 & 0.3653 \\
    Non-station. & 0.3349 & 120.245 & 1.6888 & 0.4226 & 0.3911 \\
    sinGAN & 0.3270 & 147.9333  & 1.3806 & 0.4230 &  0.3829 \\
    pix2pixHD  & 0.3253 & 131.655 &  0.5472 & 0.4193 & 0.3780 \\
    \textbf{Ours} & 0.4533 & \textbf{78.4808} & \textbf{0.3973}  & \textbf{0.3246} & \textbf{0.3563} \\
    \hline
    Non-station.$^{*}$ & \textbf{0.4915} & 211.0645 & 1.4274 & 0.3411 & 0.3893 \\
    sinGAN$^{*}$ & 0.2913 & 154.651  & 1.6909 & 0.4787 & 0.4364 \\
    DeepTexture & 0.3011 & 82.053 & 0.5649 & 0.4175 & 0.3830 \\
    WCT  & 0.3124 & 144.208 & 0.4125 & 0.4427 & 0.4068 \\
    % Ground truth &  &  &  &  & \\
    \end{tabular}
}
\vspace{2mm}
\caption{256 to 512 synthesis scores for different approaches averaged over 200 images. Non-station.$^{*}$, sinGAN$^{*}$, DeepTexture and WCT directly take the ground truth images as inputs.}
\label{tab:eval256to512}
\end{table}

\begin{figure}[h]
\centering
\scalebox{0.9}{
\addtolength{\tabcolsep}{-4pt}   
\begin{tabular}{c|cccccccc}
\multicolumn{1}{c}{} & \multicolumn{8}{c}{} \\
input & ours & Self-tuning & pix2pixHD & WCT & sinGAN$^{(*)}$ & Non-stat.$^{(*)}$ & DeepTexture & ground truth \\
\hline
\hline
\includegraphics[width=0.06\textwidth]{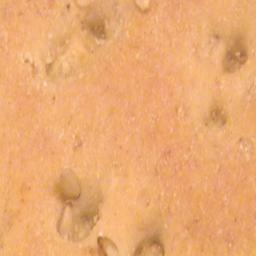} &
\includegraphics[width=0.12\textwidth]{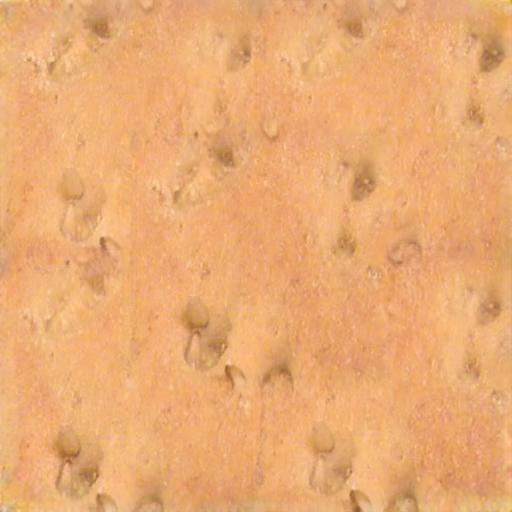} &
\includegraphics[width=0.12\textwidth]{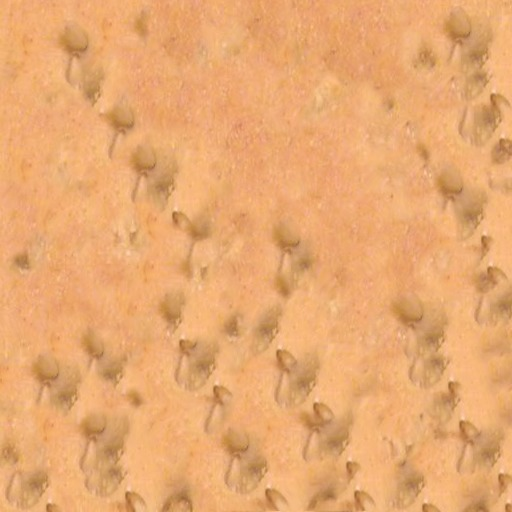} &
\includegraphics[width=0.12\textwidth]{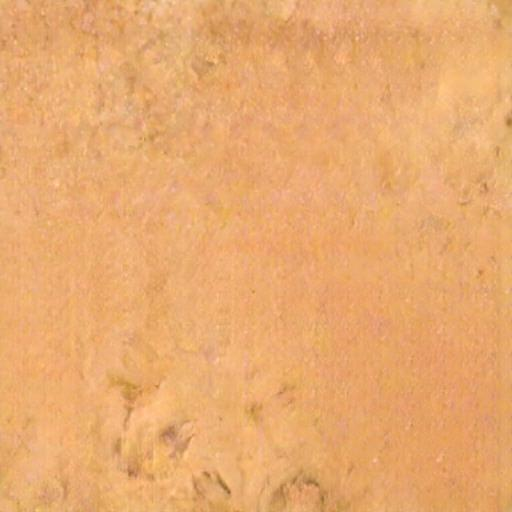} &
\includegraphics[width=0.12\textwidth]{SupplCompare512/WCT/65_c2i_iter3_alpha_100.jpg} &
\includegraphics[width=0.12\textwidth]{SupplCompare512/sinGAN_GT/65_c2i.jpg} &
\includegraphics[width=0.12\textwidth]{SupplCompare512/nonstationary_GT/65_c2i.jpg} &
\includegraphics[width=0.12\textwidth]{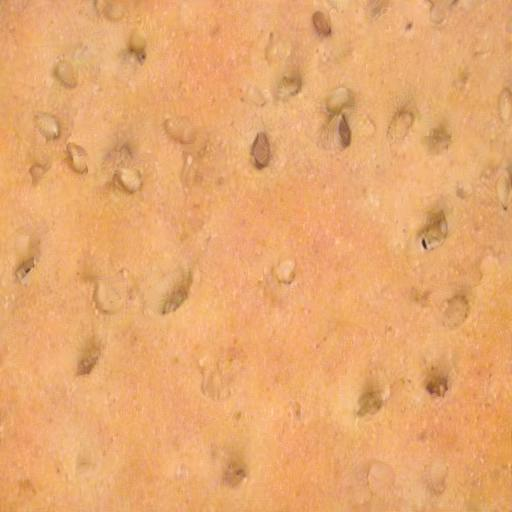} &
\includegraphics[width=0.12\textwidth]{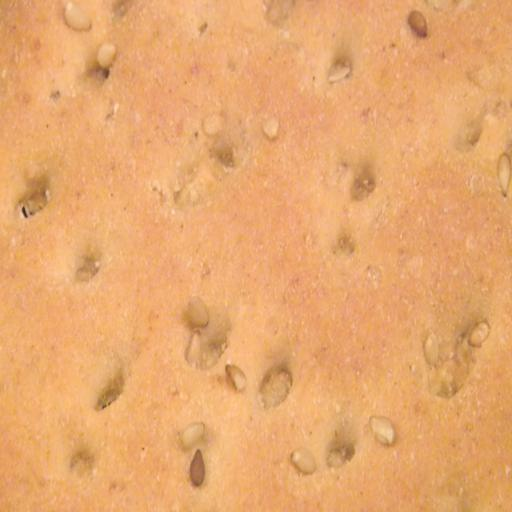} \\
\includegraphics[width=0.06\textwidth]{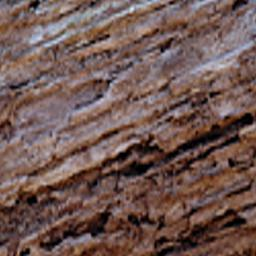} &
\includegraphics[width=0.12\textwidth]{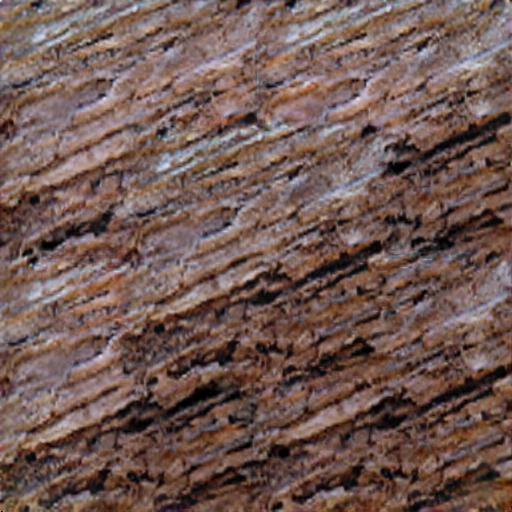} &
\includegraphics[width=0.12\textwidth]{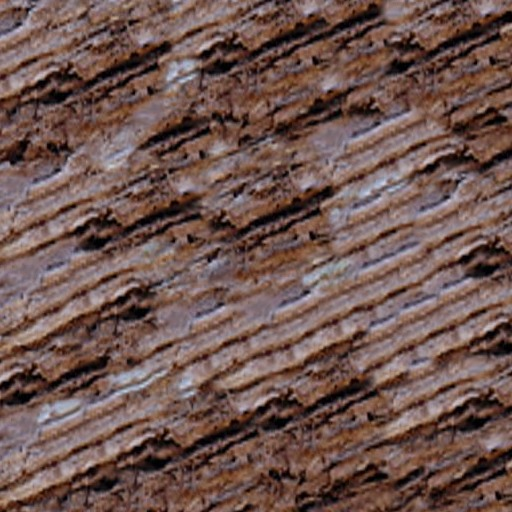} &
\includegraphics[width=0.12\textwidth]{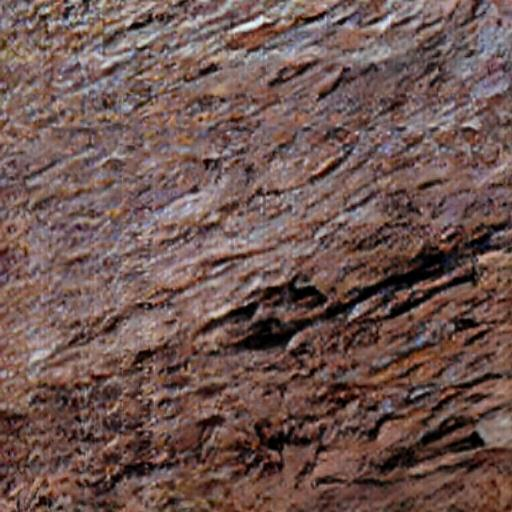} &
\includegraphics[width=0.12\textwidth]{SupplCompare512/WCT/DSC_7144_iter3_alpha_100.jpg} &
\includegraphics[width=0.12\textwidth]{SupplCompare512/sinGAN_GT/DSC_7144.jpg} &
\includegraphics[width=0.12\textwidth]{SupplCompare512/nonstationary_GT/DSC_7144.jpg} &
\includegraphics[width=0.12\textwidth]{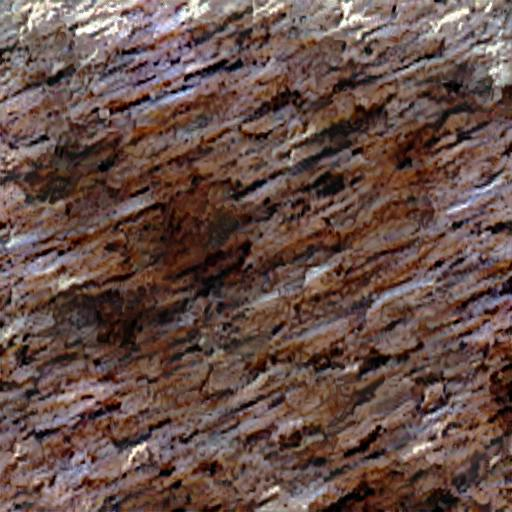} &
\includegraphics[width=0.12\textwidth]{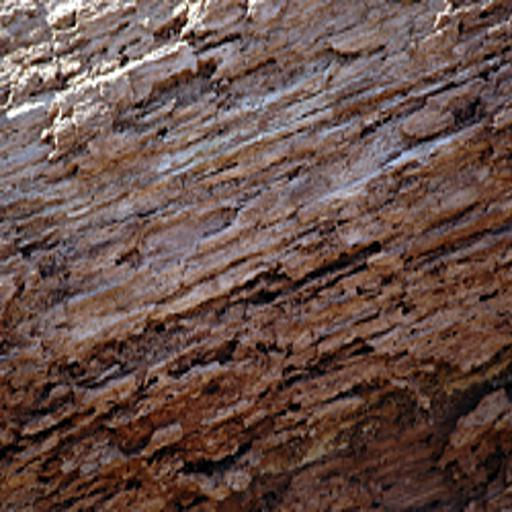} \\
\hline
\hline

\includegraphics[width=0.06\textwidth]{SupplCompare512/TransConv/21_c2l1r180_input.jpg} &
\includegraphics[width=0.12\textwidth]{SupplCompare512/TransConv/21_c2l1r180_output.jpg} &
\includegraphics[width=0.12\textwidth]{SupplCompare512/SelfTune/21_c2l1r180.jpg} &
\includegraphics[width=0.12\textwidth]{SupplCompare512/pix2pixHD/21_c2l1r180_output.jpg} &
\includegraphics[width=0.12\textwidth]{SupplCompare512/WCT/21_c2l1r180_iter3_alpha_100.jpg} &
\includegraphics[width=0.12\textwidth]{SupplCompare512/sinGAN/21_c2l1r180.jpg} &
\includegraphics[width=0.12\textwidth]{SupplCompare512/nonstationary/21_c2l1r180.jpg} &
\includegraphics[width=0.12\textwidth]{SupplCompare512/deeptexture/21_c2l1r180.jpg} &
\includegraphics[width=0.12\textwidth]{SupplCompare512/TransConv/21_c2l1r180_target.jpg} \\
\includegraphics[width=0.06\textwidth]{SupplCompare512/TransConv/193_c1l2r180_input.jpg} &
\includegraphics[width=0.12\textwidth]{SupplCompare512/TransConv/193_c1l2r180_output.jpg} &
\includegraphics[width=0.12\textwidth]{SupplCompare512/SelfTune/193_c1l2r180.jpg} &
\includegraphics[width=0.12\textwidth]{SupplCompare512/pix2pixHD/193_c1l2r180_output.jpg} &
\includegraphics[width=0.12\textwidth]{SupplCompare512/WCT/193_c1l2r180_iter3_alpha_100.jpg} &
\includegraphics[width=0.12\textwidth]{SupplCompare512/sinGAN/193_c1l2r180.jpg} &
\includegraphics[width=0.12\textwidth]{SupplCompare512/nonstationary/193_c1l2r180.jpg} &
\includegraphics[width=0.12\textwidth]{SupplCompare512/deeptexture/193_c1l2r180.jpg} &
\includegraphics[width=0.12\textwidth]{SupplCompare512/TransConv/193_c1l2r180_target.jpg} \\
\includegraphics[width=0.06\textwidth]{SupplCompare512/TransConv/226_c4l1_input.jpg} &
\includegraphics[width=0.12\textwidth]{SupplCompare512/TransConv/226_c4l1_output.jpg} &
\includegraphics[width=0.12\textwidth]{SupplCompare512/SelfTune/226_c4l1.jpg} &
\includegraphics[width=0.12\textwidth]{SupplCompare512/pix2pixHD/226_c4l1_output.jpg} &
\includegraphics[width=0.12\textwidth]{SupplCompare512/WCT/226_c4l1_iter3_alpha_100.jpg} &
\includegraphics[width=0.12\textwidth]{SupplCompare512/sinGAN/226_c4l1.jpg} &
\includegraphics[width=0.12\textwidth]{SupplCompare512/nonstationary/226_c4l1.jpg} &
\includegraphics[width=0.12\textwidth]{SupplCompare512/deeptexture/226_c4l1.jpg} &
\includegraphics[width=0.12\textwidth]{SupplCompare512/TransConv/226_c4l1_target.jpg} \\

\end{tabular}
}
\caption{Results of different approaches on 256 to 512 texture synthesis.  For sinGAN($^{*}$) Non-stat.$^{(*)}$ results, the first two rows show the results of training with ground truth; the rest rows show the results of training without ground truth. (Training with ground truth means using the ground truth 512$\times$512 image as the target for each training iteration.) WCT and DeepTexture directly take ground truth images as inputs.}
\label{fig:result512}
\end{figure}

\clearpage

\subsubsection*{128 to 512 Synthesis (4$\times$larger)}

\subsubsubsection*{Comparison to Self-tuning}

\begin{figure}[h]
\centering
\scalebox{1.0}{
\addtolength{\tabcolsep}{-4pt}  
\begin{tabular}{ccc|ccc}
% \multicolumn{1}{c}{} & \multicolumn{4}{c}{} \\
input & ours & Self-tuning & input & ours & Self-tuning \\
\includegraphics[width=0.05\textwidth]{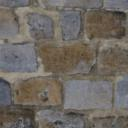}&
\includegraphics[width=0.20\textwidth]{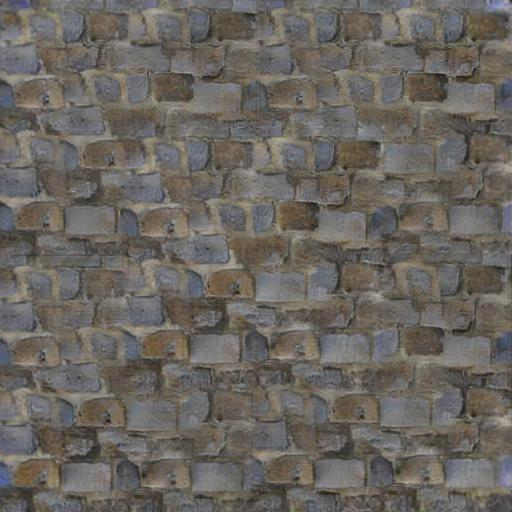}&
\includegraphics[width=0.20\textwidth]{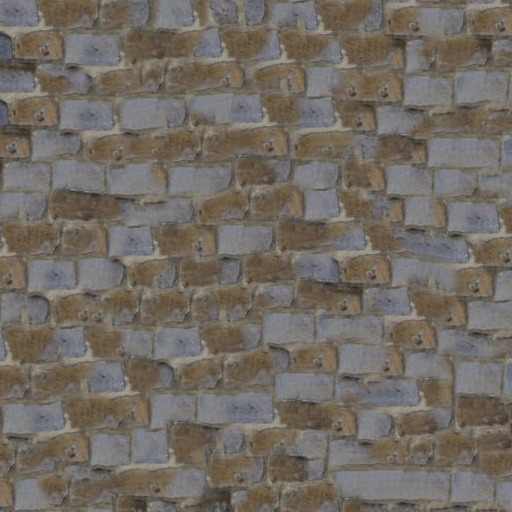} &
\includegraphics[width=0.05\textwidth]{Supple128to512/input/117_c1l2r180_input.jpg}&
\includegraphics[width=0.20\textwidth]{Supple128to512/TransConv/117_c1l2r180_target_output_output.jpg}&
\includegraphics[width=0.20\textwidth]{Supple128to512/SelfTune/117_c1l2r180_input.jpg} \\
\includegraphics[width=0.05\textwidth]{Supple128to512/input/105_c3l5r120_input.jpg}&
\includegraphics[width=0.20\textwidth]{Supple128to512/TransConv/105_c3l5r120_target_output_output.jpg}&
\includegraphics[width=0.20\textwidth]{Supple128to512/SelfTune/105_c3l5r120_input.jpg}& 
\includegraphics[width=0.05\textwidth]{Supple128to512/input/166_c3l8r120_input.jpg}&
\includegraphics[width=0.20\textwidth]{Supple128to512/TransConv/166_c3l8r120_target_output_output.jpg}&
\includegraphics[width=0.20\textwidth]{Supple128to512/SelfTune/166_c3l8r120_input.jpg} \\
\end{tabular}
}
\caption{More Comparisons between our approach and Self-tuning on 128 to 512 synthesis.}
\vspace{-0.2cm}
\end{figure}

\subsubsubsection*{Additional Results of the Proposed Method}

\begin{figure}[h]
\centering
\scalebox{0.9}{
\addtolength{\tabcolsep}{-4pt}
\begin{tabular}{cc|cc|cc|cc}
input & ours & input & ours & input & ours & input & ours \\
\includegraphics[width=0.05\textwidth]{Suppl128to512_More/84_c1l4r60_input.jpg}&
\includegraphics[width=0.2\textwidth]{Suppl128to512_More/84_c1l4r60_output_output.jpg}&
\includegraphics[width=0.05\textwidth]{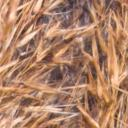}&
\includegraphics[width=0.2\textwidth]{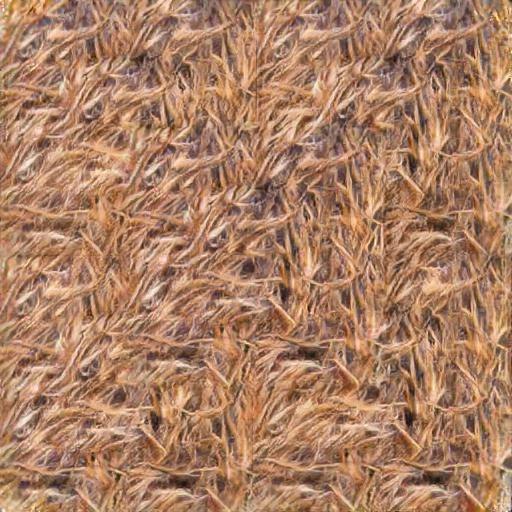}&
\includegraphics[width=0.05\textwidth]{Suppl128to512_More/1_c1l1r180_input.jpg}&
\includegraphics[width=0.2\textwidth]{Suppl128to512_More/1_c1l1r180_output_output.jpg}&
\includegraphics[width=0.05\textwidth]{Suppl128to512_More/227_c1l5r60_input.jpg}&
\includegraphics[width=0.2\textwidth]{Suppl128to512_More/227_c1l5r60_output_output.jpg}\\
\includegraphics[width=0.05\textwidth]{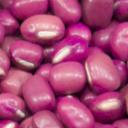}&
\includegraphics[width=0.2\textwidth]{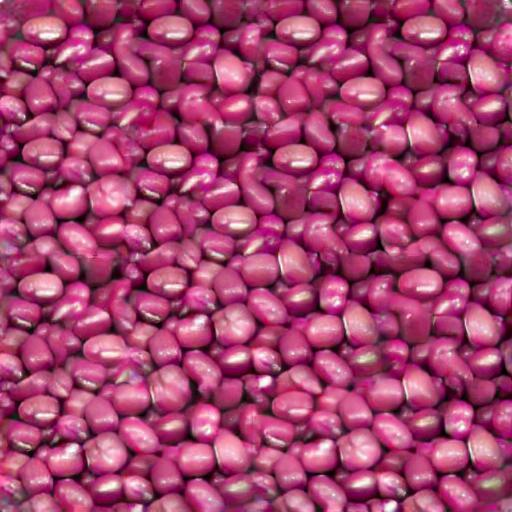}&
\includegraphics[width=0.05\textwidth]{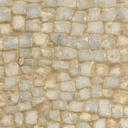}&
\includegraphics[width=0.2\textwidth]{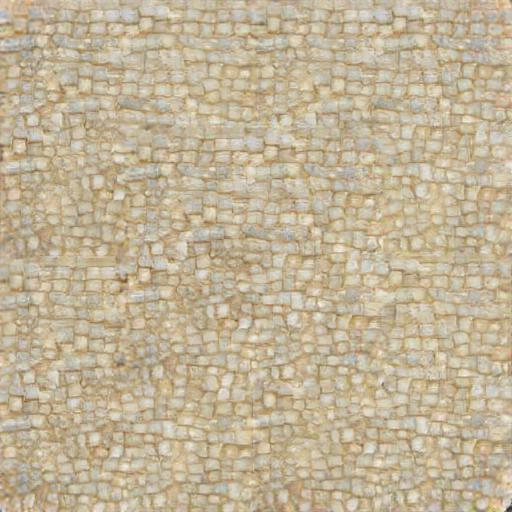}&
\includegraphics[width=0.05\textwidth]{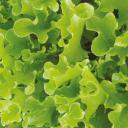}&
\includegraphics[width=0.2\textwidth]{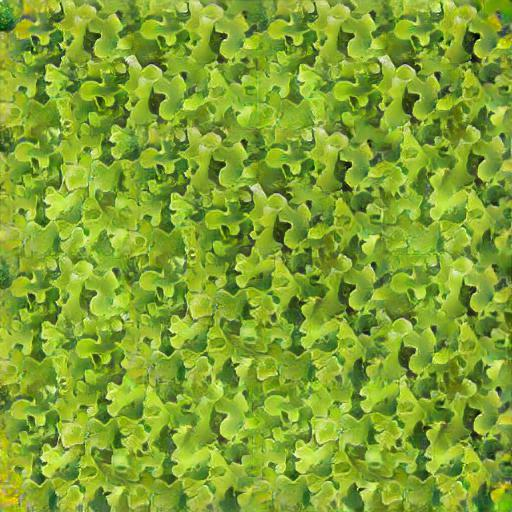}&
\includegraphics[width=0.05\textwidth]{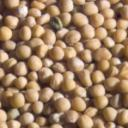}&
\includegraphics[width=0.2\textwidth]{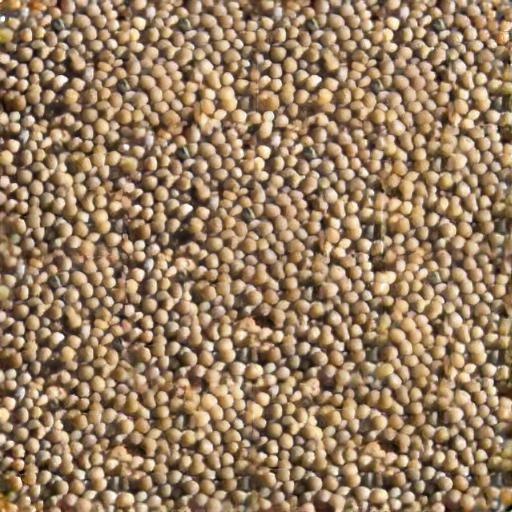}\\
\includegraphics[width=0.05\textwidth]{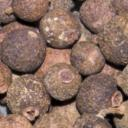}&
\includegraphics[width=0.2\textwidth]{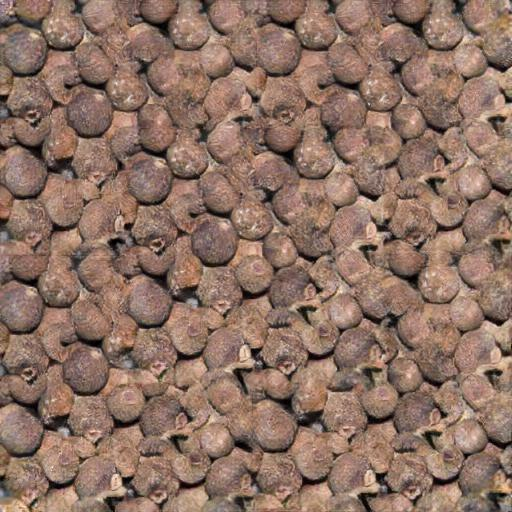}&
\includegraphics[width=0.05\textwidth]{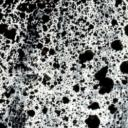}&
\includegraphics[width=0.2\textwidth]{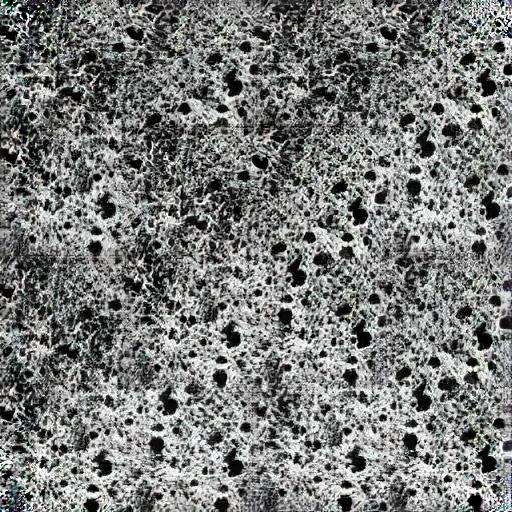}&
\includegraphics[width=0.05\textwidth]{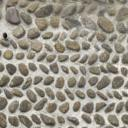}&
\includegraphics[width=0.2\textwidth]{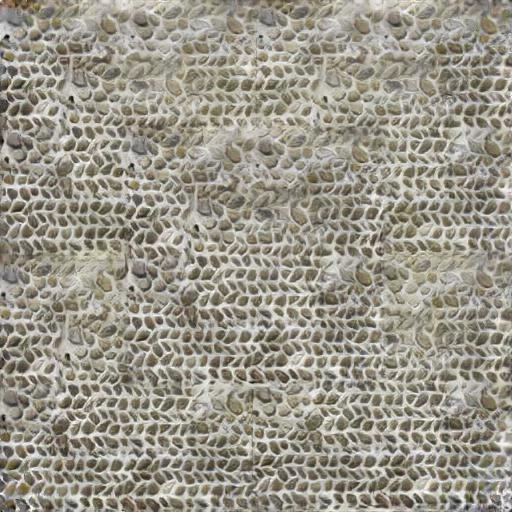}&
\includegraphics[width=0.05\textwidth]{Suppl128to512_More/Crackles0004_1_270_input.jpg}&
\includegraphics[width=0.2\textwidth]{Suppl128to512_More/Crackles0004_1_270_output_output.jpg}\\
\end{tabular}
}
\caption{More results on 128 to 512 synthesis using our method. Please zoom in for more details.}
\end{figure}
